# Supplementary material for: Temporal Representation Learning on Monocular Videos for 3D Human Pose Estimation
Source: arXiv:2012.01511 source file (2022-11-25)
Supplement: Supplementary file 2 [file supp_dive_pose5.tex]

% !TEX root = ../cvpr.tex
% !TEX spellcheck = en-US

\begin{figure*}[t]
	\centering
	\includegraphics[width=1\textwidth]{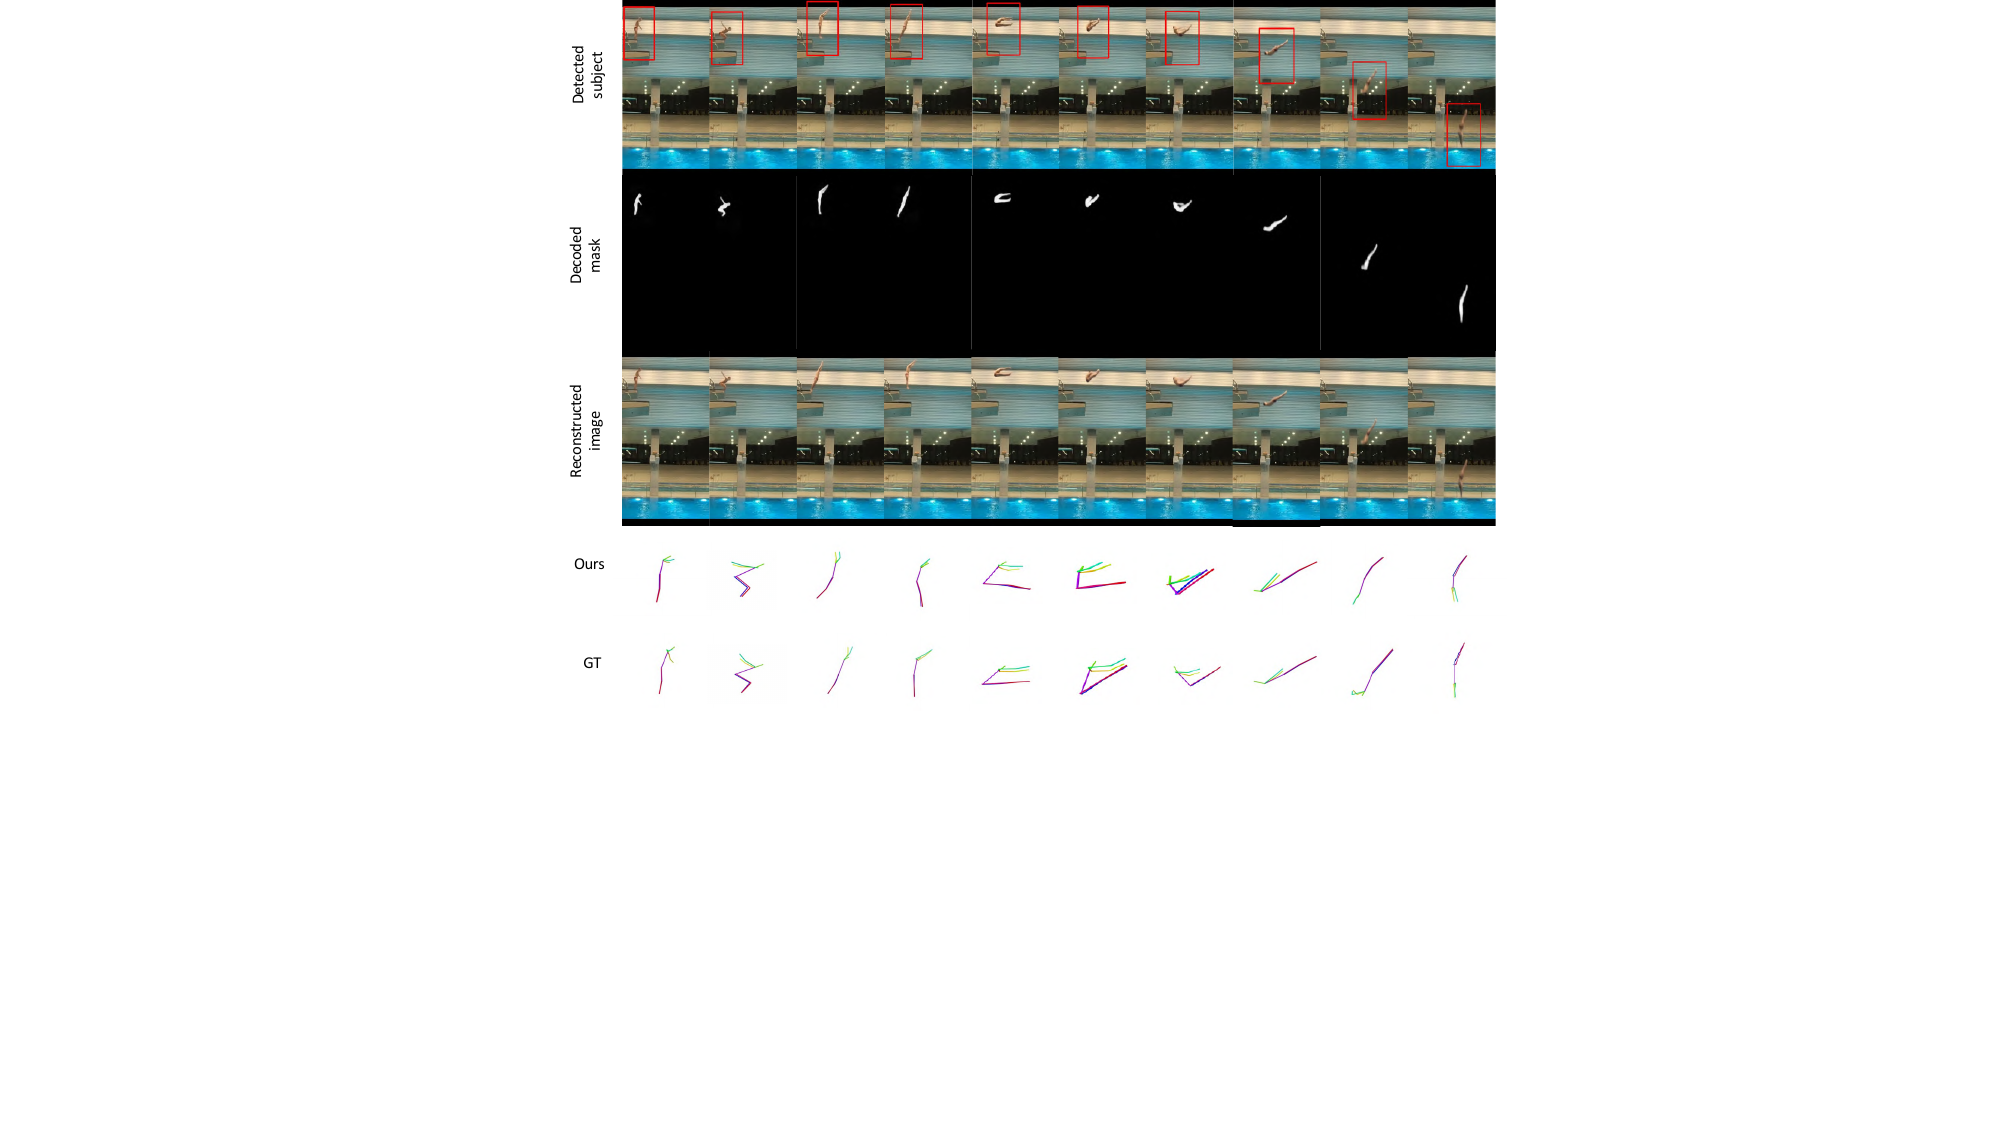}
	\caption{\small {\bf Qualitative results on Diving Dataset}.  
		Samples are taken from the test set. In the top row, the red  rectangle shows the bounding box detected by our model for image cropping. The second and third rows, show respectively the decoded mask and re-synthesized image. Bottom rows show the pose estimation of our approach and the GT labels.
	}
	\label{fig:supp_dive_pose5}
	\vspace{1cm}
\end{figure*}
